# Supplementary material for: 3D simulations of wet foam coarsening evidence a self similar growth regime
Source: arXiv:1502.03366 source file (2015-02-11)
Supplement: Supplementary file 1 [file Suppl_COLSUA-D-14-01513R2.pdf]

# Supplementary materials for 3D simulations of wet foam coarsening evidence a self similar growth regime

Gilberto L. Thomas[a], Julio M. Belmonte[b,c], François Graner[d], James A. Glazier[c], Rita M.C. de Almeida[a,c,e,*]

[a]*Instituto de Física, Universidade Federal do Rio Grande do Sul Av. Bento Gonçalves 9500, C.P. 15051 - 91501-970 Porto Alegre, RS, Brazil*
[b]*European Molecular Biology Laboratory Heidelberg, Meyerhofstr. 1, 69117 Heidelberg, Germany*
[c]*Biocomplexity Institute and Department of Physics, Indiana University Bloomington, Vloomington, Indiana, 47405-7105, United States of America*
[d]*Matière et Systèmes Complexes, Université Paris Diderot, CNRS UMR 7057, 10 rue Alice Domon et Léonie Duquet, F-75205 Paris Cedex 13, France*
[e]*Instituto Nacional de Ciência e Tecnologia - Sistemas Complexos Av. Bento Gonçalves 9500, C.P. 15051 - 91501-970 Porto Alegre, RS, Brazil*

*Email: rita@if.ufrgs.br, Tel: +555133086521, Fax: +5533087286

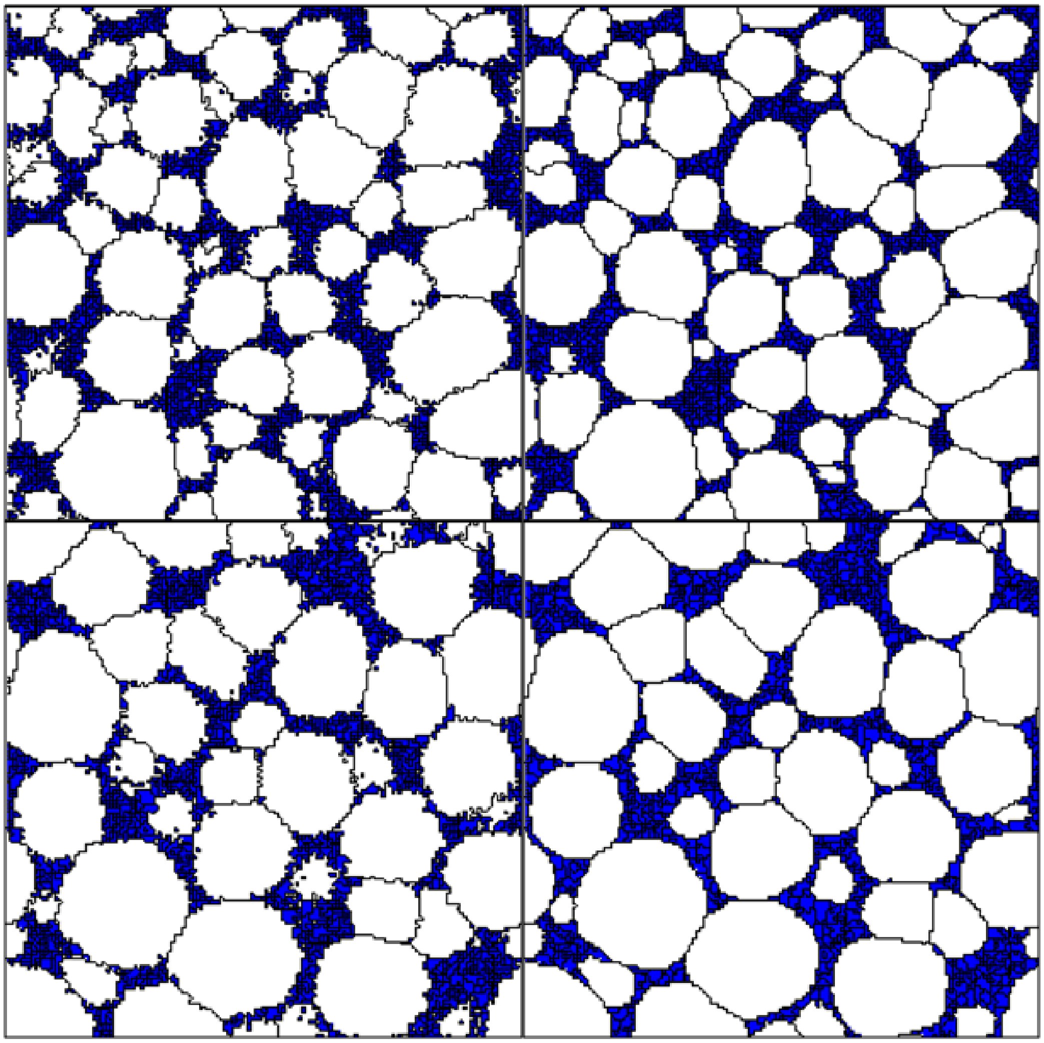

Figure 1: Fluid particles: 2D slices of 3D simulations around 3000 MCS, during self-similar growth, for $\phi = 0.20$ and $V^{target} = 10$ voxels (top) and 50 voxels (bottom). Left: Before interface relaxation. Right: After interface relaxation.

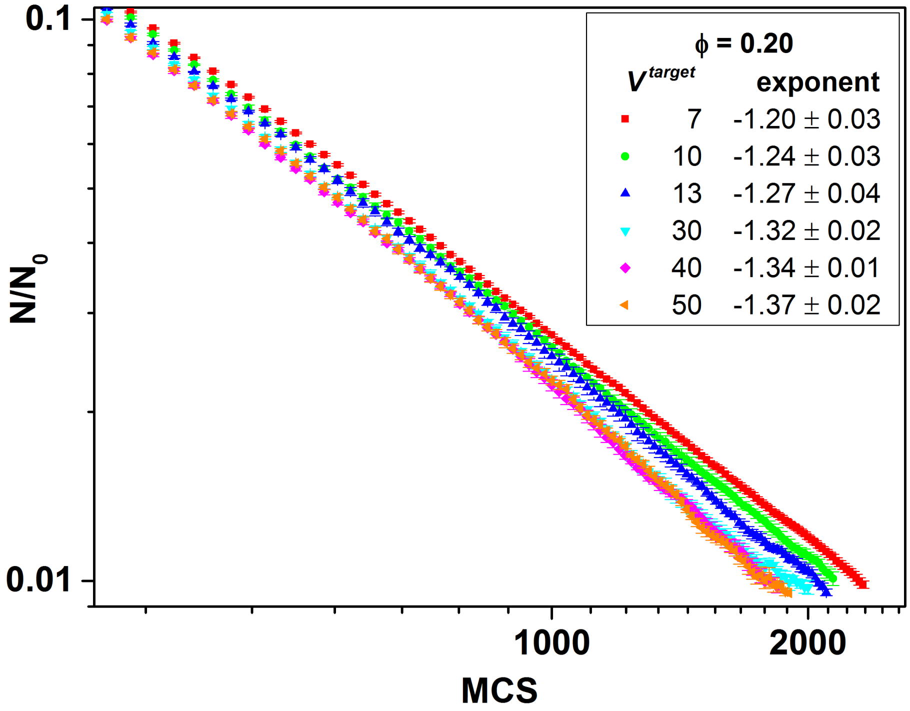


Figure 2: Effect of the target volume of fluid particles ($V^{target}$) on foam evolution: Log-log plot of the number of bubbles vs time for $\phi = 0.20$ in a $150^3$ grid, starting from a log-normal bubble volume distribution. Curves are averaged over 5 simulation replicas for $\lambda_{liq} = 70$, and $J$s are as described in Eq. (2). The growth exponent increases as $V^{target}$ increases.

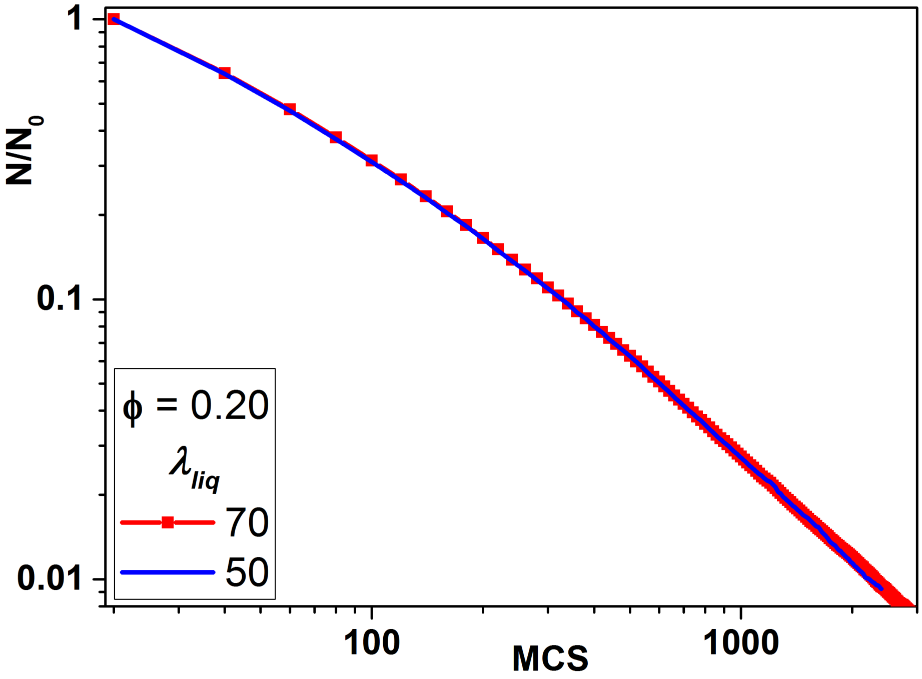


Figure 3: Effect of the fluid particle compression modulus, $\lambda_{liq}$: Log-log plot of the number of bubbles vs time for $\phi = 0.20$ in a $150^3$ grid, starting from a log-normal bubble volume distribution. Curves are averaged over 5 simulation replicas for $\lambda_{liq} = 50$ and 70, and $J$s are as described in Eq. (2). Changing the modulus has no significant effect on the growth exponent.

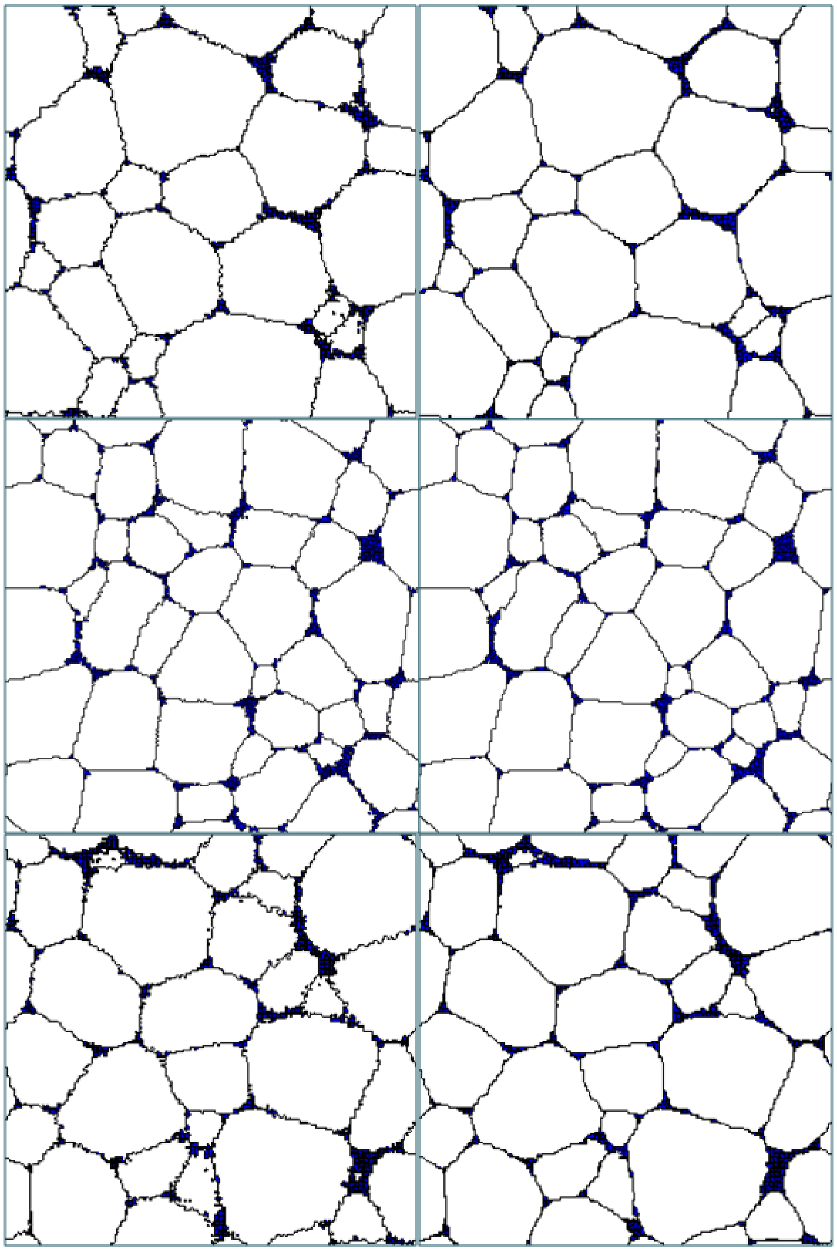

Figure 4: 2D slices of 3D simulations around 3000 MCS, in the self-similar regime, for $\phi = 0.05$ and $J(gas, gas) = 1.9$, 1.99, and 1.999 (from top to bottom, respectively). Left: Before interface relaxation. Right: After interface relaxation.

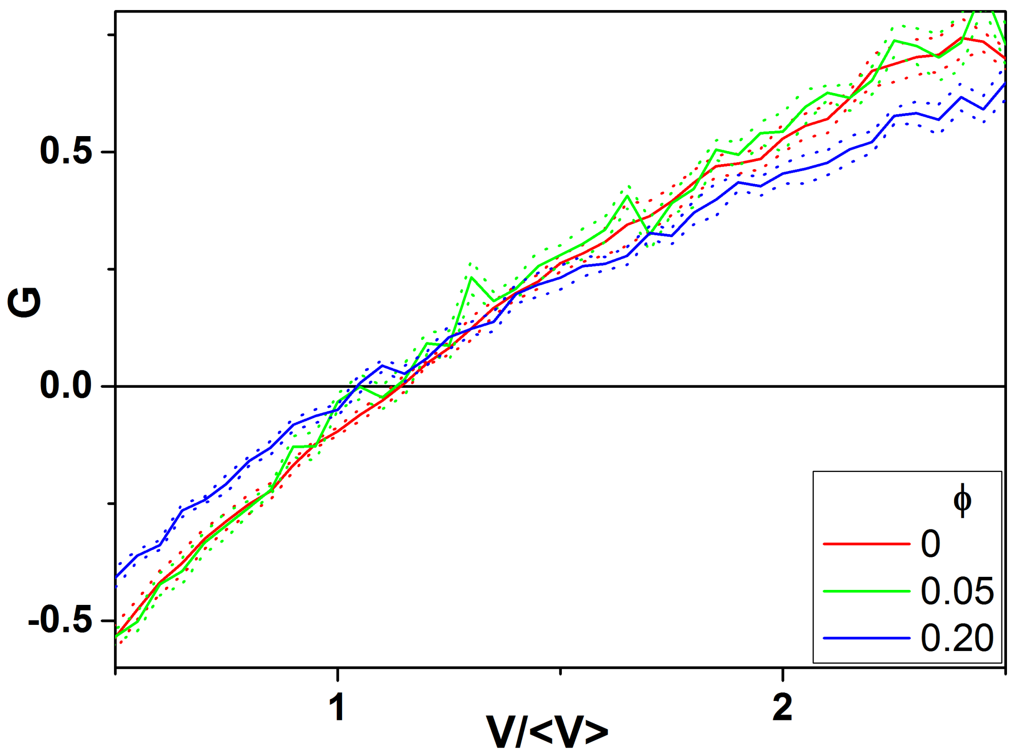


Figure 5: Detail of figure 5 (lower panel) showing the different growth rates for different foam wetnesses.

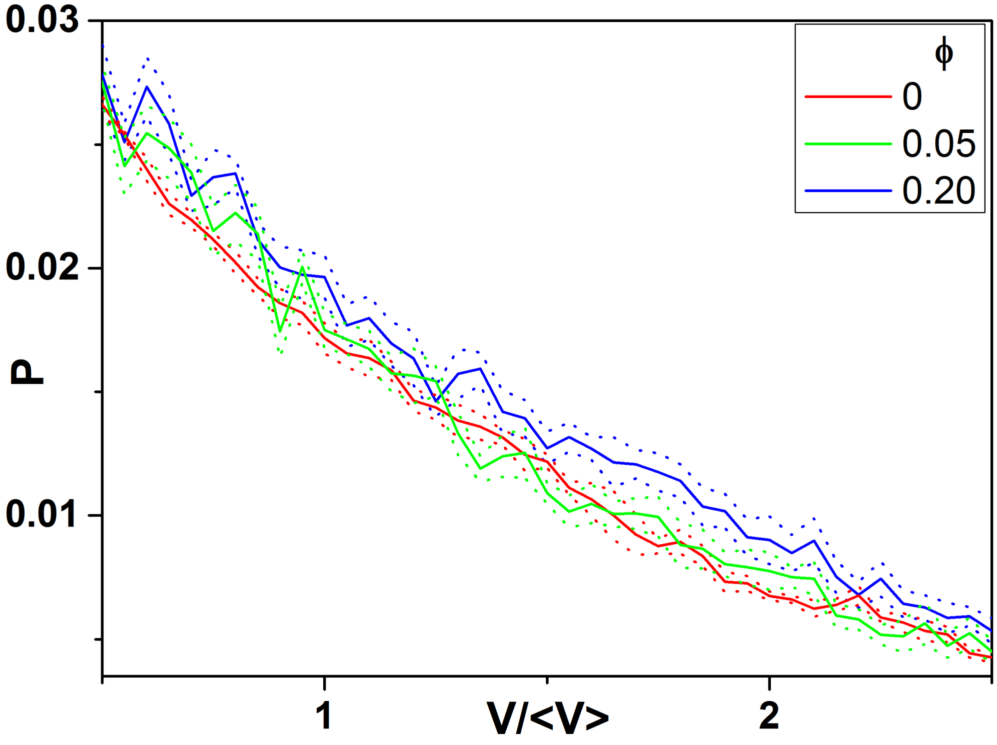


Figure 6: Detail of figure 6 (lower panel) showing the different self-similar volume distributions for different foam wetnesses.

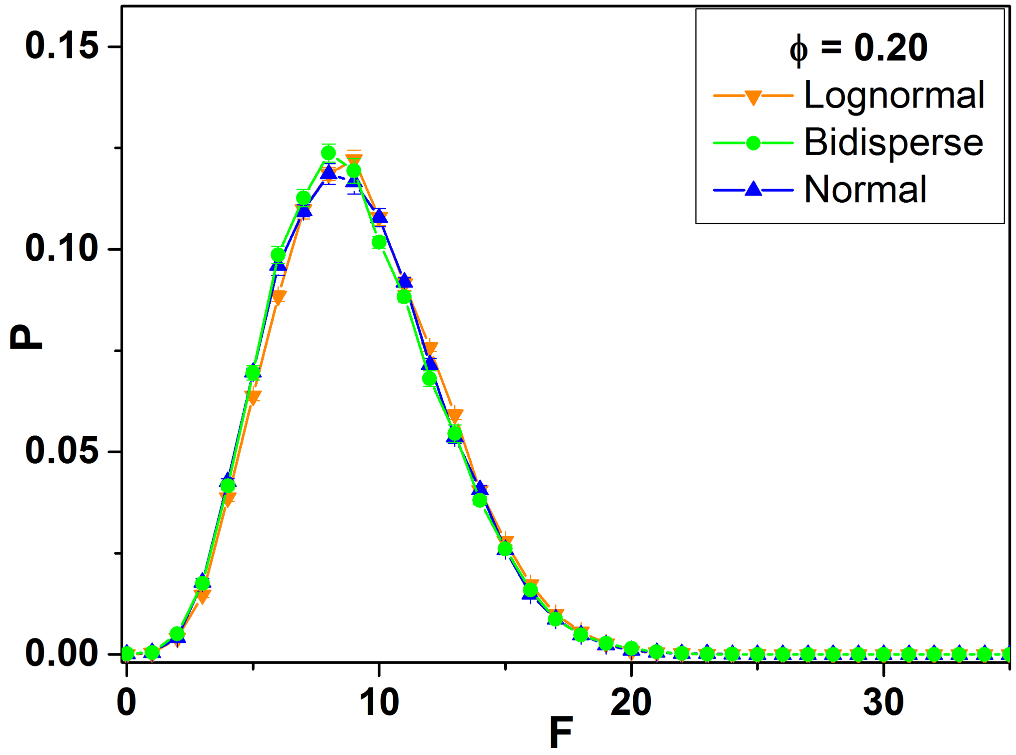


Figure 7: Probability distributions for number of faces $F$ for different initial bubble-volume distributions for $\phi = 0.20$.
